# Supplementary material for: Learning to Count without Annotations
Source: arXiv:2307.08727 source file (2024-03-29)
Supplement: Supplementary file 1 [file appendix_qualitative.pdf]

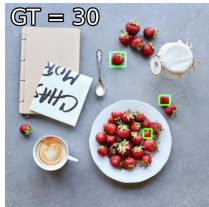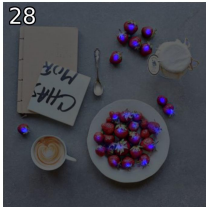

(a) GT=30; Pred=28

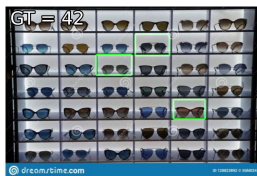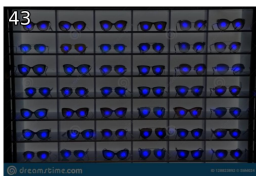

(b) GT=42; Pred=43

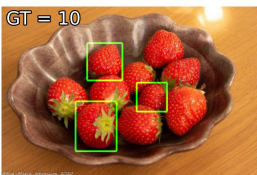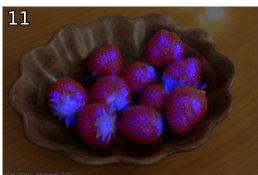

(c) GT=10; Pred=11

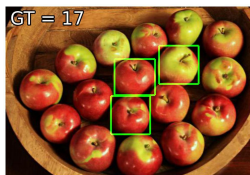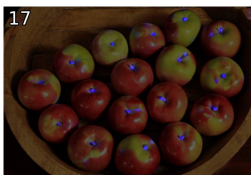

(d) GT=17; Pred=17

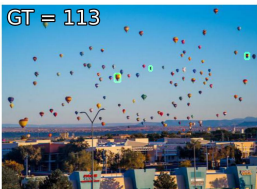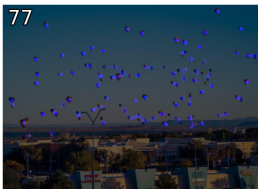

(e) GT=113; Pred=77

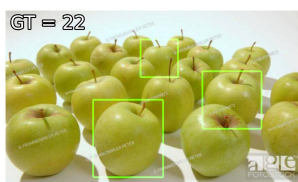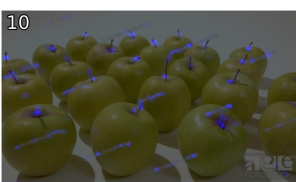

(f) GT=22; Pred=10

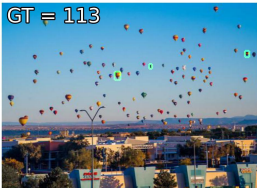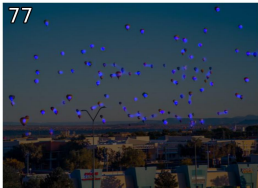

(a) GT=113; Pred=77

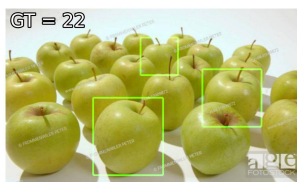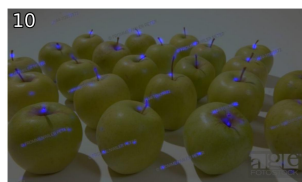

(b) GT=22; Pred=10

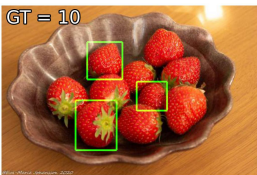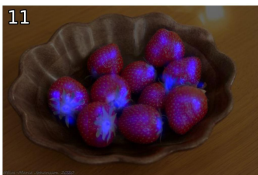

(c) GT=10; Pred=11

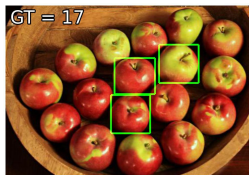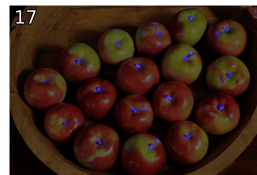

(d) GT=17; Pred=17

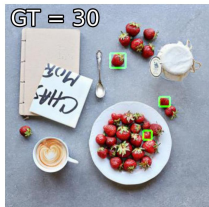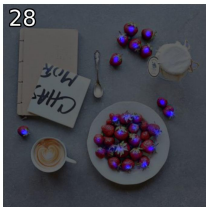

(e) GT=30; Pred=28

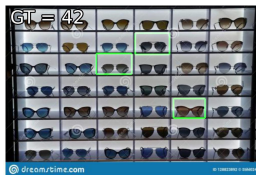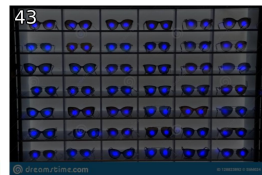

(f) GT=42; Pred=43
